# Supplementary material for: AFF-ttention! Affordances and Attention models for Short-Term Object Interaction Anticipation
Source: arXiv:2406.01194 source file (2024-06-05)
Supplement: Supplementary file 1 [file supp.tex]

\setcounter{page}{1}
\title{AFF-ttention! Affordances and Attention models \\ for Short-Term Object Interaction Anticipation \\(Supplementary Material)}
\maketitle 

\noindent
This document reports additional experimental details which could not be included in the main paper due to space limits. 

\section{Datasets}

We validate our method on Ego4D~\cite{grauman2022ego4d} and EPIC-Kitchens~\cite{damen2018scaling}, two large-scale datasets of egocentric videos with high diversity and long-tail distributions of verbs and nouns classes.

\paragraph{\textbf{Ego4D}}
We consider both the first and second versions of Ego4D STA annotations. Version 1 (v1) of the Ego4D STA split is composed of 27,801 training 17,217 validation and 19,870 test instances with 87 noun and 74 verb categories. Version 2 (v2) extends v1 with additional videos and annotations, for a total of 98,276 training, 47,385 validation and 19,870 test videos, with a taxonomy of 128 nouns and 81 verb classes. Ego4D STA contains a single test split which is compatible with v1 and v2, hence models trained on either versions can be compared on the same test split, with methods trained on v2 generally performing better thanks to the extended annotations.

\paragraph{\textbf{EPIC-Kitchens}}
Since Ego4D is the only dataset containing STA annotations to date, we contribute a second benchmark by extending over action and object annotations available in the popular EPIC-Kitchens dataset~\cite{damen2018scaling}. 
The extended annotations are obtained by post-processing and filtering existing active object and action segment annotations available in the EPIC-KITCHENS dataset.
STA annotations are obtained in four stages.
In the first stage, we process active object bounding box annotations to form object tracks. This is done by merging in the same track neighbouring annotations related to the same object class.
Since annotators have been instructed to label all instances of the active object (e.g., all instances of ``plate``), we removed all tracks containing frames with more than one labeled bounding box for the same object class.
In the second stage, each object track is matched to one of the annotated action segments. Specifically, if an action segment including the same noun as the object track is found, this is matched to the object track.
In the third stage, we truncate object tracks so that they do not include the action. This is done because we are interested in anticipating the future action, which hence should not be observed.
In the fourth stage, we attach the following data to a given bounding box: the noun associated to the track as the object category, the of the associated action segment as the interaction verb, the distance from the timestep of the current frame to the beginning of the associated action segment as the time to contact.
The final set of annotations contains 33,804 training and 7,055 validation instances with 104 noun and 51 verb categories. Annotations will be publicly released to encourage future research. 

\section{Implementation details}

\paragraph{\textbf{Training details}}

We train the STAformer classifier with Adam as an optimizer, an initial learning rate of $10^{-4}$ with linear warm-up, and a weight decay of $10^{-6}$, on 4 Tesla V100 GPUs. For both datasets, we sample 16 frames at 30 frames per second to form the input video clips, which are downscaled to a height of 320 pixels. We follow the standard Faster-RCNN resolutions and resize the short side in the range $[$640, 672, 704, 736, 768, 800 $]$ with a maximum long side of 1333. We use the DINOv2 "base" version composed of 12 blocks and an embedding space of 768 channels. Following previous work \cite{izquierdo2023optimal}, we only fine-tune the last 3 blocks. We initialize the TimeSformer weights with the dual encoder version of EgoVLP-v2 \cite{pramanick2023egovlpv2} pre-trained on EgoClip \cite{lin2022egocentric}. We interpolate the spatial and temporal positional encoding of TimeSformer to adapt the video processing resolution, established in 224 $\times$ 336.

\paragraph{\textbf{STA Prediction head}}

We adopt the prediction head proposed in~\cite{ragusa2023stillfast}, which modifies the Faster-RCNN~\cite{girshick2015fast} head integrating components specialized for STA prediction. In short, the fused feature pyramid $P_T$ (Figure 2.d) is passed to a Region Proposal Network (RPN), which computes object proposals. Such proposals are then used to extract local features from $P_T$ with RoI Align~\cite{he2017mask}, mapping bounding boxes to appropriate layers of the pyramid following~\cite{lin2017feature}. Each extracted local feature vector is concatenated with the fused class token $C_T$ (Figure 2.c) and passed through an MLP with a residual connection. Linear layers are used to compute noun probabilities $p(n)_i$, verb probabilities $p(v)_i$ and time-to-contact (ttc) predictions.

\paragraph{\textbf{Extracting environment affordances zones}}
To build the affordance database we follow Algorithm 1 from \cite{nagarajan2020ego} to define zones, but omit adding edges between zones. This algorithm compares the similarity between two frames with a pre-trained Siamesse neural network composed by a Resnet-18 \cite{he2016deep} followed by a 5 layer multi-layer perceptron (MLP). Previously, we select similar/dissimilar frames for the training labels. We consider two similar frames if they were separated less than 15 frames or they share 10 inlier homography key-points. We extract SuperPoint keypoint descriptors \cite{detone2018superpoint} for the homography estimation. We measure the visual similarity from pre-trained ResNet-152 features \cite{he2016deep} to select dissimilar frames.

\paragraph{\textbf{Leveraging interaction hotspots:}}
On the interaction hotspots model, we fine-tune the hands detector by Shan et al. \cite{shan2020understanding} with the annotations present at the Object State Change detection (SCOD) split of Ego4D. We remove from the SCOD training split those scenes present at the STA validation splits. 

\section{Extra results}

\paragraph{\textbf{Ablation study on Environment Affordances}}

\begin{table}[t]
\centering
\caption{Ablation study on different configurations of the environment affordances performance on the Ego4D-STA v1, using a StillFast architecture as base model.}
\begin{tabular}{|ccc|c|c|c|c|}
        \hline 
        K(text) & K(video) &Dist. &  N&  N+V& N+$\delta$&All\\ \hline
        \multicolumn{3}{|c|}{No affordances}& 16.20& 7.47& 4.94&2.48\\ \hline
 \multicolumn{3}{|c|}{Ego-Topo \cite{nagarajan2020ego}}& 14.92& 6.45& 4.01&2.14\\ \hline 
             top-4& -& U& 17.64 & 8.05 & 5.13 & 2.58\\
             -&    top-4& U& 17.98 & 7.95 & 5.19 & 2.67 \\ 
                  top-4& top-4& U& 18.27& 8.24& 5.35&2.71\\ \hline
             top-2& top-2&W& 17.90& 7.77& 5.34&2.65\\ 
             top-4& top-4&W& 18.44& \textbf{8.52}& 5.46&\textbf{2.85}\\ 
             top-6& top-6&W& \textbf{18.75}& 8.46& \textbf{5.47}&2.81\\
             top-8& top-8&W& 18.53& 8.40& 5.45&2.76\\\hline
\end{tabular}
\label{tab:env_aff_supp}
\end{table}

Table \ref{tab:env_aff_supp} compares the performance of StillFast when using different environment affordance configurations as priors. Compared with training an NN using the affordances as ground-truth for supervision as in \cite{nagarajan2020ego} does not improve the final performance after fusing the measurements. Our intuition is that the NN learns almost the same interactions as the STA classifier and therefore it does not improve when both are fused and loses the generalist quality of our approach. First, we evaluate the influence of the visual and cross similarity when selecting the K-Nearest Neighbours (NN). As the results show, the combined version obtains the best performance (18.27 N, 8.24 N+V, 5.35 N+$\delta$ and 2.71 All). This indicates that visual similarity is not enough in a cultural-diverse dataset like Ego4D, where the same action can be performed in multiple different environments. Second, we weigh the influence of each zone affordance distribution according to its respective similarity. This version obtains a minor improvement up to 18.44 N, 8.52 N+V, 5.47 N+$\delta$ and 2.85 Overall. Finally, we analyze the influence of the number of considered zones at the K-NN. Keeping a low number of zones reduces the affordance richness and makes it more difficult for the next interaction to falls inside, while increasing the number of considered zones creates a wider affordance distribution but dilutes the STA value. 

\paragraph{\textbf{Visualization of Environment affordances nodes}}

We illustrate in Figures \ref{fig:ego4d_aff} and \ref{fig:ek_aff} some environmental affordances zones extracted from Ego4D and EPIC-Kitchens, respectively. Each row shows different frames that compose the zone captured at different moments of the sequence, representing an activity-centric region like \textit{washing the dishes, ironing, unboxing a package, taking fresh food...}.

\begin{figure}
\centering

\includegraphics[width=0.19\textwidth]{imgs_E4D/a01.png}
\includegraphics[width=0.19\textwidth]{imgs_E4D/a02.png}
\includegraphics[width=0.19\textwidth]{imgs_E4D/a03.png}
\includegraphics[width=0.19\textwidth]{imgs_E4D/a04.png} 
\includegraphics[width=0.19\textwidth]{imgs_E4D/a05.png}\\

\includegraphics[width=0.19\textwidth]{imgs_E4D/b01.png}
\includegraphics[width=0.19\textwidth]{imgs_E4D/b02.png}
\includegraphics[width=0.19\textwidth]{imgs_E4D/b03.png}
\includegraphics[width=0.19\textwidth]{imgs_E4D/b04.png} 
\includegraphics[width=0.19\textwidth]{imgs_E4D/b05.png}\\

\includegraphics[width=0.19\textwidth]{imgs_E4D/c01.png}
\includegraphics[width=0.19\textwidth]{imgs_E4D/c02.png}
\includegraphics[width=0.19\textwidth]{imgs_E4D/c03.png}
\includegraphics[width=0.19\textwidth]{imgs_E4D/c04.png} 
\includegraphics[width=0.19\textwidth]{imgs_E4D/c05.png}\\

\includegraphics[width=0.19\textwidth]{imgs_E4D/d01.png}
\includegraphics[width=0.19\textwidth]{imgs_E4D/d02.png}
\includegraphics[width=0.19\textwidth]{imgs_E4D/d03.png}
\includegraphics[width=0.19\textwidth]{imgs_E4D/d04.png} 
\includegraphics[width=0.19\textwidth]{imgs_E4D/d05.png}\\

\includegraphics[width=0.19\textwidth]{ECCV_2024_Lorenzo/imgs_E4D/brush1.png}
\includegraphics[width=0.19\textwidth]{ECCV_2024_Lorenzo/imgs_E4D/brush2.png}
\includegraphics[width=0.19\textwidth]{ECCV_2024_Lorenzo/imgs_E4D/brush3.png}
\includegraphics[width=0.19\textwidth]{ECCV_2024_Lorenzo/imgs_E4D/bursh4.png} 
\includegraphics[width=0.19\textwidth]{ECCV_2024_Lorenzo/imgs_E4D/bursh5.png}\\

\includegraphics[width=0.19\textwidth]{imgs_E4D/f01.png}
\includegraphics[width=0.19\textwidth]{imgs_E4D/f02.png}
\includegraphics[width=0.19\textwidth]{imgs_E4D/f03.png}
\includegraphics[width=0.19\textwidth]{imgs_E4D/f04.png} 
\includegraphics[width=0.19\textwidth]{imgs_E4D/f05.png}\\

\includegraphics[width=0.19\textwidth]{imgs_E4D/h01.png}
\includegraphics[width=0.19\textwidth]{imgs_E4D/h02.png}
\includegraphics[width=0.19\textwidth]{imgs_E4D/h03.png}
\includegraphics[width=0.19\textwidth]{imgs_E4D/h04.png} 
\includegraphics[width=0.19\textwidth]{imgs_E4D/h05.png}\\

\includegraphics[width=0.19\textwidth]{imgs_E4D/i01.png}
\includegraphics[width=0.19\textwidth]{imgs_E4D/i02.png}
\includegraphics[width=0.19\textwidth]{imgs_E4D/i03.png}
\includegraphics[width=0.19\textwidth]{imgs_E4D/i06.png} 
\includegraphics[width=0.19\textwidth]{imgs_E4D/i05.png}\\

\caption{Zones of the environment affordances database extracted in Ego4D following \cite{nagarajan2020ego}. Each row corresponds to a single node representing an activity-centric region.}
\label{fig:ego4d_aff}
\end{figure}

\begin{figure}
\centering

\includegraphics[width=0.19\textwidth]{imgs_EK/p01_b1.png}
\includegraphics[width=0.19\textwidth]{imgs_EK/p01_b2.png}
\includegraphics[width=0.19\textwidth]{imgs_EK/p01_b3.png}
\includegraphics[width=0.19\textwidth]{imgs_EK/p01_b4.png} 
\includegraphics[width=0.19\textwidth]{imgs_EK/p01_b5.png}\\

\includegraphics[width=0.19\textwidth]{imgs_EK/p01_d1.png}
\includegraphics[width=0.19\textwidth]{imgs_EK/p01_d2.png}
\includegraphics[width=0.19\textwidth]{imgs_EK/p01_d3.png}
\includegraphics[width=0.19\textwidth]{imgs_EK/p01_d4.png} 
\includegraphics[width=0.19\textwidth]{imgs_EK/p01_d5.png}\\

\includegraphics[width=0.19\textwidth]{imgs_EK/p02_b1.png}
\includegraphics[width=0.19\textwidth]{imgs_EK/p02_b2.png}
\includegraphics[width=0.19\textwidth]{imgs_EK/p02_b3.png}
\includegraphics[width=0.19\textwidth]{imgs_EK/p02_b4.png} 
\includegraphics[width=0.19\textwidth]{imgs_EK/p02_b5.png}\\

\includegraphics[width=0.19\textwidth]{imgs_EK/p03_a5.png}
\includegraphics[width=0.19\textwidth]{imgs_EK/p03_a2.png}
\includegraphics[width=0.19\textwidth]{imgs_EK/p03_a3.png}
\includegraphics[width=0.19\textwidth]{imgs_EK/p03_a4.png} 
\includegraphics[width=0.19\textwidth]{imgs_EK/p03_a1.png}\\

\includegraphics[width=0.19\textwidth]{imgs_EK/p01_a1.png}
\includegraphics[width=0.19\textwidth]{imgs_EK/p01_a2.png}
\includegraphics[width=0.19\textwidth]{imgs_EK/p01_a3.png}
\includegraphics[width=0.19\textwidth]{imgs_EK/p01_a4.png} 
\includegraphics[width=0.19\textwidth]{imgs_EK/p01_a2.png}\\

\includegraphics[width=0.19\textwidth]{imgs_EK/p05_a1.png}
\includegraphics[width=0.19\textwidth]{imgs_EK/p05_a3.png}
\includegraphics[width=0.19\textwidth]{imgs_EK/p05_a4.png}
\includegraphics[width=0.19\textwidth]{imgs_EK/p05_a5.png} 
\includegraphics[width=0.19\textwidth]{ECCV_2024_Lorenzo/imgs_EK/p05_a2.png}\\

\includegraphics[width=0.19\textwidth]{imgs_EK/p07_a1.png}
\includegraphics[width=0.19\textwidth]{imgs_EK/p07_a2.png}
\includegraphics[width=0.19\textwidth]{imgs_EK/p07_a3.png}
\includegraphics[width=0.19\textwidth]{imgs_EK/p07_a4.png} 
\includegraphics[width=0.19\textwidth]{imgs_EK/p07_a5.png}\\

\includegraphics[width=0.19\textwidth]{imgs_EK/p01_e1.png}
\includegraphics[width=0.19\textwidth]{imgs_EK/p01_e2.png}
\includegraphics[width=0.19\textwidth]{imgs_EK/p01_e3.png}
\includegraphics[width=0.19\textwidth]{imgs_EK/p01_e4.png} 
\includegraphics[width=0.19\textwidth]{imgs_EK/p01_e2.png}

\caption{Zones of the environment affordances database extracted in EK following \cite{nagarajan2020ego}. Each row corresponds to a single node representing an activity-centric region.}
\label{fig:ek_aff}
\end{figure}

\paragraph{\textbf{Interaction hotspots results}}

\begin{figure}
\centering
\includegraphics[width=\textwidth]{images/hands_gt_1.jpg}
\caption{Hands trajectory along the seen video, obtained by finetunned a hand object detector on Ego4D sequences}
\label{fig:hands_traj}
\end{figure}

\begin{table}[t]
    \centering
    \begin{minipage}{0.49\linewidth}
        \caption{Object interaction hotspots performance on the Ego4D-STA v1.}    \centering
        \begin{tabular}{|c|c|c|c|} \hline 
             &  SIM&  AUC-Judd&  NSS\\ \hline 
              
 Hotspots \cite{nagarajan2019grounded}&   0.309&  0.665&  0.145\\ \hline 
 LOCATE \cite{li2023locate}&  0.324&  0.641&  0.258\\ \hline 
 Join hands \cite{liu2022joint}& 0.652& 0.806 & 1.305\\\hline 
 Join hands  (ours)&  \textbf{0.672}&  \textbf{0.832}&  \textbf{1.421}\\ \hline
        \end{tabular}
        \label{tab:int_hotspots_baselines}
    \end{minipage}
    \hfill
    \begin{minipage}{0.49\linewidth}
    \centering
        \caption{Hands detection Average Precision (AP) score on the Ego4D SCOD v1.}
        \begin{tabular}{|c|c|c|c|} \hline 
             &  AP25&  AP50&  AP75 \\ \hline 
             Zisserman \cite{zhang2023helping} &    0.781&  0.567&  0.487 \\ \hline 
             Sha et al. \cite{shan2020understanding} \faSnowflake&    0.874&   0.855&   0.751 \\ \hline 
             Sha et al. \cite{shan2020understanding} \faWrench&  \textbf{0.931} & \textbf{0.906} & \textbf{0.783} \\ \hline
        \end{tabular}
        \vspace{3 mm}
        \label{tab:hands_results}
    \end{minipage}
\end{table}

We compare in Table \ref{tab:int_hotspots_baselines} the performance of different baselines on the interaction hotspots prediction. We obtain minor improvements (0.672 vs 0.652 SIM, 0.832 vs 0.806 AUC-Judd, and 1.421 vs 1.305) on the model by Liu et al.  \cite{liu2022joint} with features pre-extracted with EgoVLP and refined bounding boxes obtained with a fine-tunned version of Sha et al. \cite{shan2020understanding} hand objects detector. We report in Table \ref{tab:hands_results} the effect of fine-tuning the hands detector on the AP on the Ego4D - State Change Object Detection (SCOD) validation split hand bounding box labels.

\section{Qualitative results}

We show in Figures \ref{fig:supp_ql_EGO4D} qualitative examples of the STA predictions on Ego4D. Figure \ref{fig:supp_ql_EK55} illustrates our curated STA annotations and predictions on EPIC-Kitchens. The model predicts several next-active objects, showing multiple plausible scenarios and the challenges associated to the task.

\begin{figure}[H]
    \centering
    \includegraphics[width=0.32\textwidth]{ECCV_2024_Lorenzo/SUPP_QL/Screenshot from 2024-03-01 15-51-02.png}
    \hfill
    \includegraphics[width=0.32\textwidth]{ECCV_2024_Lorenzo/SUPP_QL/Screenshot from 2024-03-01 15-51-14.png}
    \hfill
    \includegraphics[width=0.32\textwidth]{ECCV_2024_Lorenzo/SUPP_QL/Screenshot from 2024-03-01 15-51-25.png}
    \\
    \centering
    \includegraphics[width=0.32\textwidth]{ECCV_2024_Lorenzo/SUPP_QL/Screenshot from 2024-03-01 15-51-42.png}
    \hfill
    \includegraphics[width=0.32\textwidth]{ECCV_2024_Lorenzo/SUPP_QL/Screenshot from 2024-03-01 15-51-51.png}
    \hfill
    \includegraphics[width=0.32\textwidth]{ECCV_2024_Lorenzo/SUPP_QL/Screenshot from 2024-03-01 15-52-01.png}
    \\
    \centering
    \includegraphics[width=0.32\textwidth]{ECCV_2024_Lorenzo/SUPP_QL/Screenshot from 2024-03-01 15-52-23.png}
    \hfill
    \includegraphics[width=0.32\textwidth]{ECCV_2024_Lorenzo/SUPP_QL/Screenshot from 2024-03-01 15-52-35.png}
    \hfill
    \includegraphics[width=0.32\textwidth]{ECCV_2024_Lorenzo/SUPP_QL/Screenshot from 2024-03-01 15-54-45.png}
    \\
    \centering
    \includegraphics[width=0.32\textwidth]{ECCV_2024_Lorenzo/SUPP_QL/Screenshot from 2024-03-01 15-59-15.png}
    \hfill
    \includegraphics[width=0.32\textwidth]{ECCV_2024_Lorenzo/SUPP_QL/Screenshot from 2024-03-01 15-58-19.png}
    \hfill
    \includegraphics[width=0.32\textwidth]{ECCV_2024_Lorenzo/SUPP_QL/Screenshot from 2024-03-01 15-56-28.png}
    \\
    \centering
    \includegraphics[width=0.32\textwidth]{ECCV_2024_Lorenzo/SUPP_QL/Screenshot from 2024-03-01 15-54-59.png}
    \hfill
    \includegraphics[width=0.32\textwidth]{ECCV_2024_Lorenzo/SUPP_QL/Screenshot from 2024-03-01 15-56-03.png}
    \hfill
    \includegraphics[width=0.32\textwidth]{ECCV_2024_Lorenzo/SUPP_QL/Screenshot from 2024-03-01 15-59-05.png}
    \\
    \centering
    \includegraphics[width=0.32\textwidth]{ECCV_2024_Lorenzo/imgs_E4D/final_e4d_1.png}
    \hfill
    \includegraphics[width=0.32\textwidth]{ECCV_2024_Lorenzo/imgs_E4D/final_e4d2.png}
    \hfill
    \includegraphics[width=0.32\textwidth]{ECCV_2024_Lorenzo/imgs_E4D/final_e4d3.png}
    \\
   
    \caption{Qualitative results on Ego4D}
    \label{fig:supp_ql_EGO4D}
\end{figure}

\begin{figure}[H]
    \centering
    \includegraphics[width=0.32\textwidth]{ECCV_2024_Lorenzo/EK_ql/ek_gt_new_1.png}
    \hfill
    \includegraphics[width=0.32\textwidth]{ECCV_2024_Lorenzo/EK_gt/salad_corrected.png}
    \hfill
    \includegraphics[width=0.32\textwidth]{ECCV_2024_Lorenzo/EK_gt/ek_gt_12.png}
    \\
    \centering
    \includegraphics[width=0.32\textwidth]{ECCV_2024_Lorenzo/EK_ql/ek_ql_17.png}
    \hfill
    \includegraphics[width=0.32\textwidth]{ECCV_2024_Lorenzo/EK_ql/ek_ql_19.png}
    \hfill
    \includegraphics[width=0.32\textwidth]{ECCV_2024_Lorenzo/EK_ql/ek_ql_12.png}
    
    \\
    \vspace{2 mm}
    \\

    \centering
    \includegraphics[width=0.32\textwidth]{ECCV_2024_Lorenzo/EK_ql/ek_gt_new_5.png}
    \hfill
    \includegraphics[width=0.32\textwidth]{ECCV_2024_Lorenzo/EK_gt/ek_gt_6.png}
    \hfill
    \includegraphics[width=0.32\textwidth]{ECCV_2024_Lorenzo/EK_gt/ek_gt_7.png}  
    \\
    \centering
    \includegraphics[width=0.32\textwidth]{ECCV_2024_Lorenzo/EK_ql/ek_ql_5.png}
    \hfill
    \includegraphics[width=0.32\textwidth]{ECCV_2024_Lorenzo/EK_ql/ek_ql_6.png}
    \hfill
    \includegraphics[width=0.32\textwidth]{ECCV_2024_Lorenzo/EK_ql/ek_ql_7.png}
    
    \\
    \vspace{2 mm}
    \\
    
    \centering
    \includegraphics[width=0.32\textwidth]{ECCV_2024_Lorenzo/EK_gt/ek_gt_9.png}
    \hfill
    \includegraphics[width=0.32\textwidth]{ECCV_2024_Lorenzo/EK_gt/ek_gt_10.png}
    \hfill
    \includegraphics[width=0.32\textwidth]{ECCV_2024_Lorenzo/EK_gt/ek_gt_11.png}
    \\
    \centering
    \includegraphics[width=0.32\textwidth]{ECCV_2024_Lorenzo/EK_ql/ek_ql_9.png}
    \hfill
    \includegraphics[width=0.32\textwidth]{ECCV_2024_Lorenzo/EK_ql/ek_ql_10.png}
    \hfill
    \includegraphics[width=0.32\textwidth]{ECCV_2024_Lorenzo/EK_ql/ek_ql_11.png}
    
    \\
    \vspace{2 mm}
    \\
    
    \centering
    \includegraphics[width=0.32\textwidth]{ECCV_2024_Lorenzo/EK_gt/new_gt_13.png}
    \hfill
    \includegraphics[width=0.32\textwidth]{ECCV_2024_Lorenzo/EK_gt/ek_gt_14.png}
    \hfill
    \includegraphics[width=0.32\textwidth]{ECCV_2024_Lorenzo/EK_gt/ek_gt_15.png}
    \\
    \centering
    \includegraphics[width=0.32\textwidth]{ECCV_2024_Lorenzo/EK_ql/ek_ql_20.png}
    \hfill
    \includegraphics[width=0.32\textwidth]{ECCV_2024_Lorenzo/EK_ql/ek_ql_14.png}
    \hfill
    \includegraphics[width=0.32\textwidth]{ECCV_2024_Lorenzo/EK_ql/ek_ql_15.png}

    \caption{STA curated labels (top) and qualitative results (bottom) on EK}
    \label{fig:supp_ql_EK55}
\end{figure}

\begin{figure}[H]
    \centering
    \includegraphics[width=0.19\textwidth]{ECCV_2024_Lorenzo/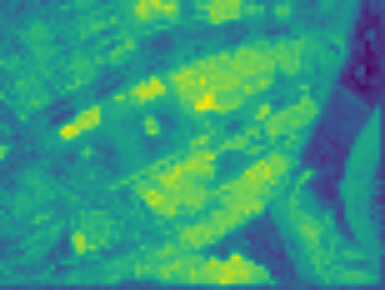}
    \hfill
    \includegraphics[width=0.19\textwidth]{ECCV_2024_Lorenzo/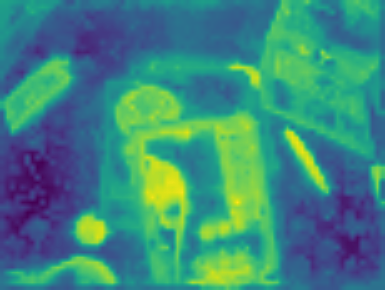}
    \hfill
    \includegraphics[width=0.19\textwidth]{ECCV_2024_Lorenzo/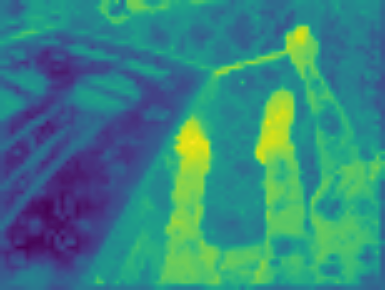}
    \hfill
    \includegraphics[width=0.19\textwidth]{ECCV_2024_Lorenzo/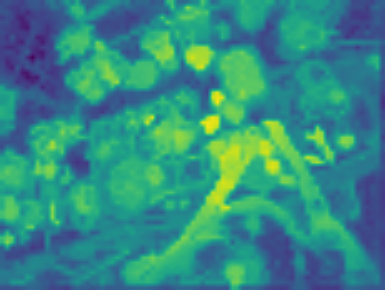}
    \hfill
    \includegraphics[width=0.19\textwidth]{ECCV_2024_Lorenzo/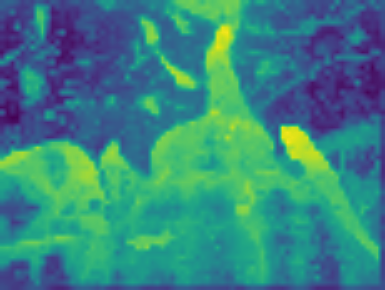}
    
    \\
    \centering
    \includegraphics[width=0.19\textwidth]{ECCV_2024_Lorenzo/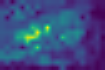}
    \hfill
    \includegraphics[width=0.19\textwidth]{ECCV_2024_Lorenzo/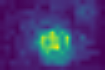}
    \hfill
    \includegraphics[width=0.19\textwidth]{ECCV_2024_Lorenzo/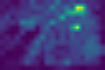}
    \hfill
    \includegraphics[width=0.19\textwidth]{ECCV_2024_Lorenzo/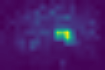}
    \hfill
    \includegraphics[width=0.19\textwidth]{ECCV_2024_Lorenzo/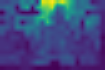}
    
    \\
    \centering
    \includegraphics[width=0.19\textwidth]{ECCV_2024_Lorenzo/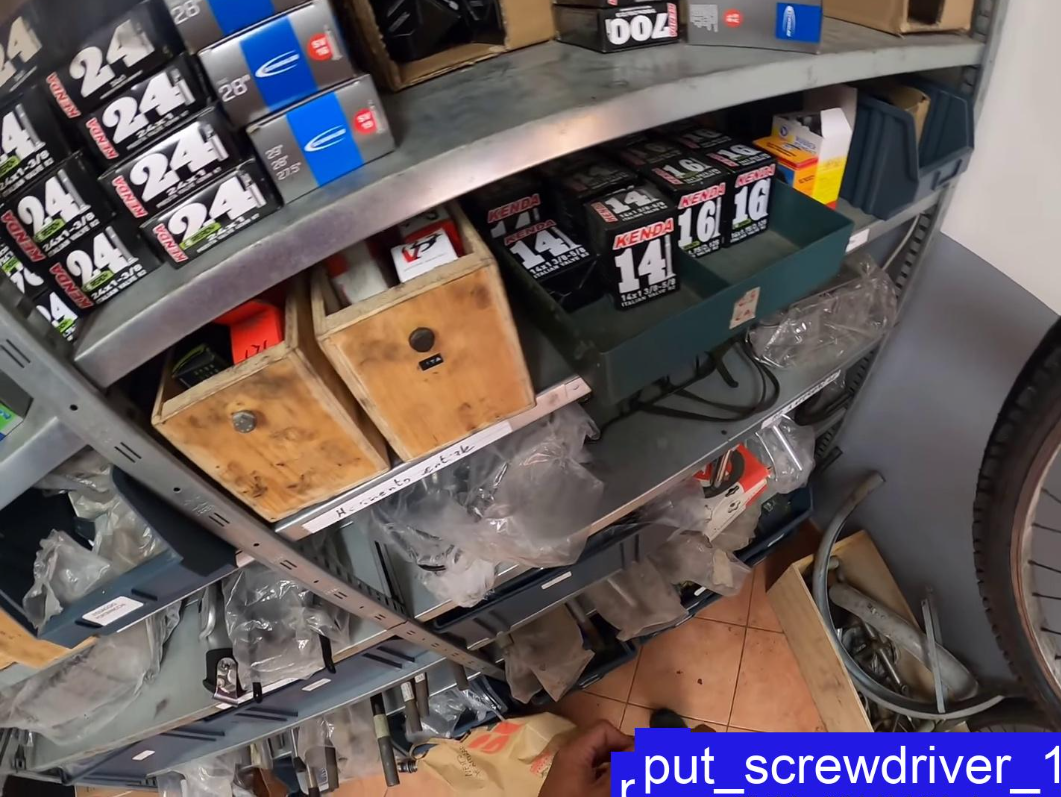}
    \hfill
    \includegraphics[width=0.19\textwidth]{ECCV_2024_Lorenzo/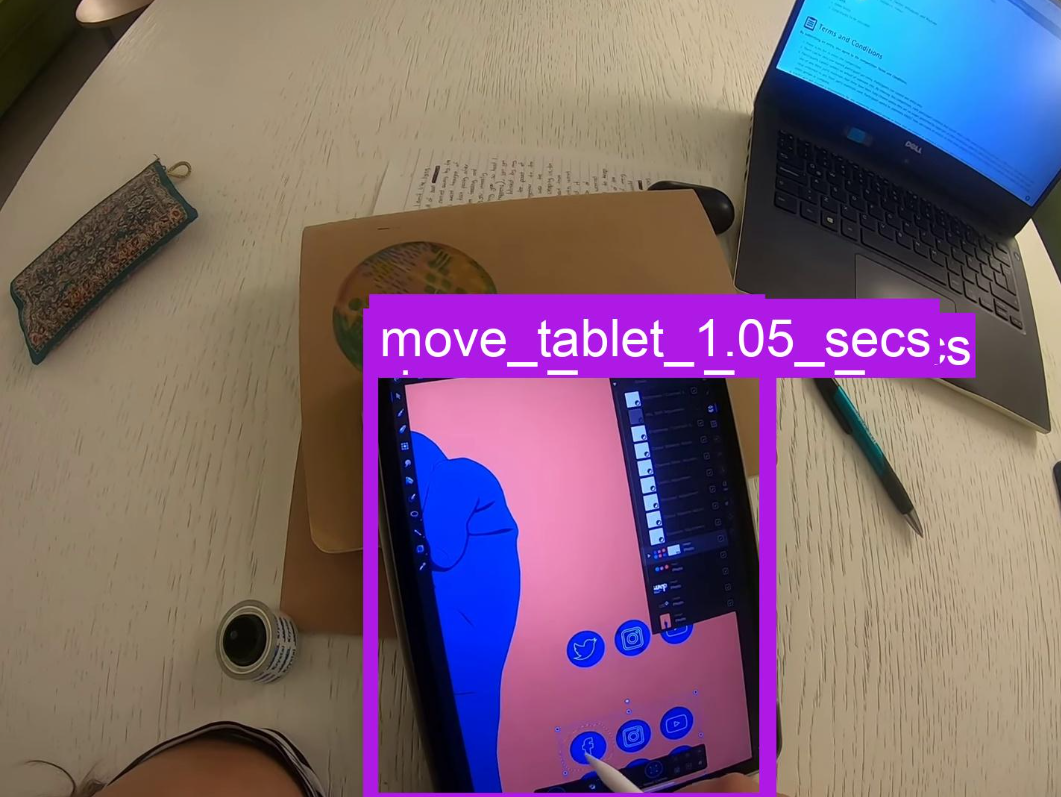}
    \hfill
    \includegraphics[width=0.19\textwidth]{ECCV_2024_Lorenzo/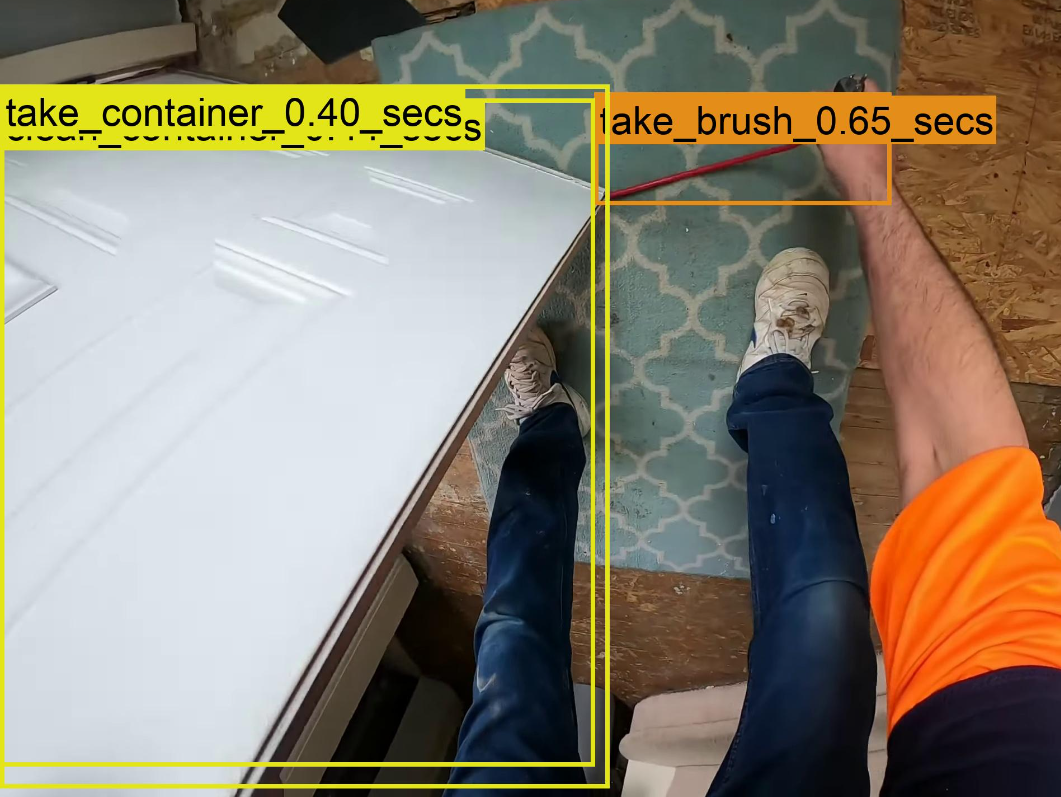}
    \hfill 
    \includegraphics[width=0.19\textwidth]{ECCV_2024_Lorenzo/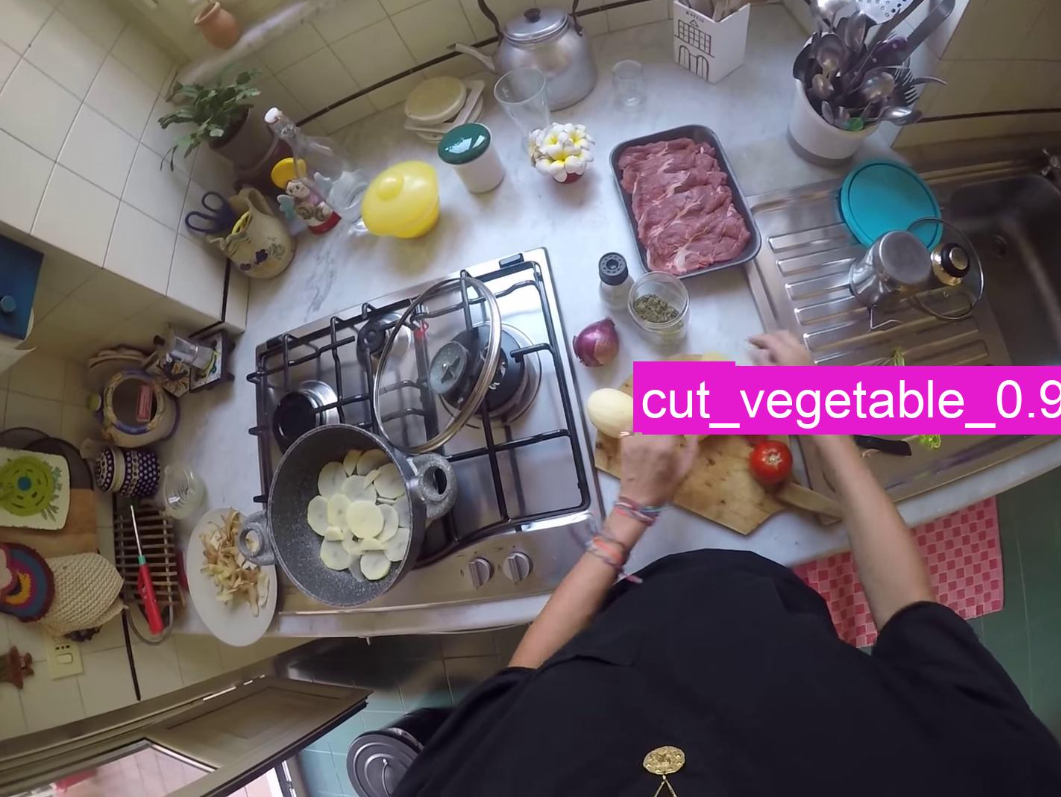}
    \hfill
    \includegraphics[width=0.19\textwidth]{ECCV_2024_Lorenzo/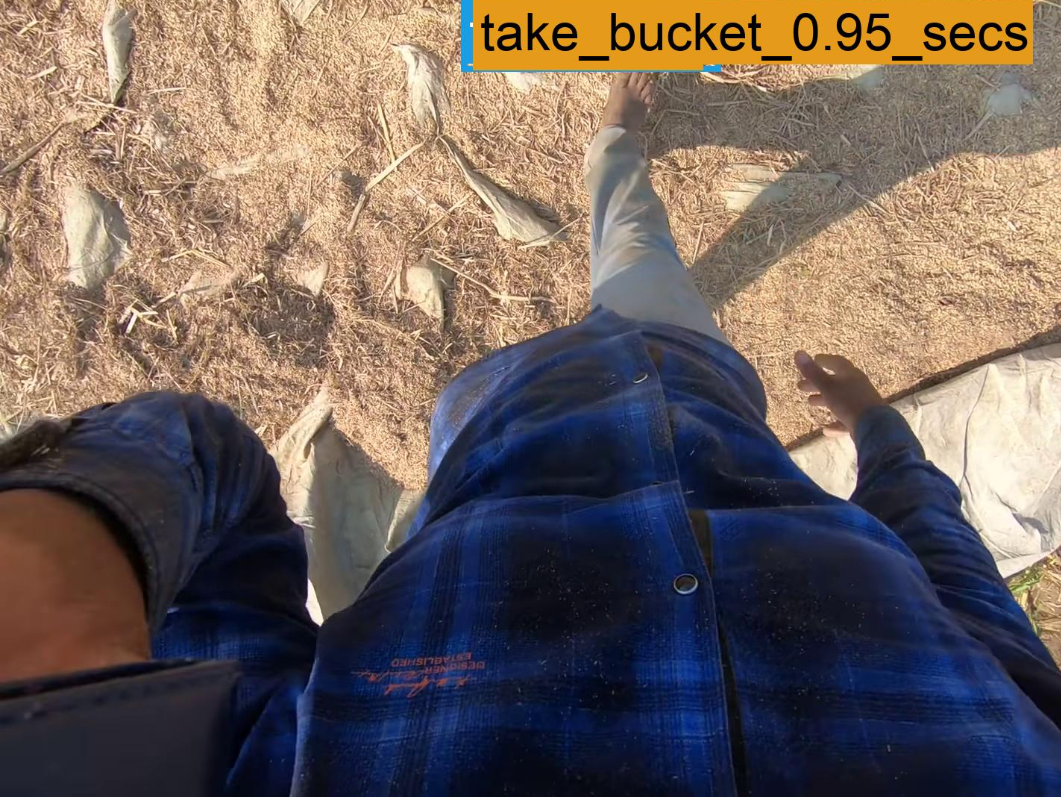}
    \\
    
    \caption{\textbf{Qualitative results and dual cross-attention maps}. We show the attention map of the video on the image features (top), the attention map of the image on the video features (middle) and the result of the final predictions. }
    \label{fig:supp_attention_maps}
\end{figure}

\begin{figure}[H]
    \centering
    \includegraphics[width=0.99\textwidth]{ECCV_2024_Lorenzo/EK_gt/LEADERBOARD.png}
    
    \caption{\textbf{EGO 4D STA Leaderboard}}
    \label{fig:imagenes_lado_a_lado}
\end{figure}

\paragraph{\textbf{Attention maps}}

The attention maps reflects the different parts of the scene attended by at the Dual Cross Attention mechanism. On top, we appreciate how the video features are refined with high-resolution details from the image, like the small vegetables on the fourth column. In the middle, we show the parts of the video more relevant for the static image, which correspond to moving regions associated with the hands motions very informative for the upcoming interaction, like the third column example. In the last row, we show the result of the predictions.

\subsection{STA Leaderboard}

Our team, called "Zarrio", scores first on the Ego4D STA leaderboard a the submission date. The reported version is trained on the version 2 of Ego4D and incorporates the affordances refinement on the STAformer predictions.
